# Supplementary material for: Anomalous cooling and heating - the Mpemba effect and its inverse
Source: arXiv:1609.05271 source file (2016-09-17)
Supplement: Supplementary file 1 [file GeneralizedMpemba_SI.pdf]

# Supplementary Information: Anomalous cooing and heating – the Mpemba effect and its inverse

Zhiyue Lu[1] and Oren Raz[2]

[1] James Franck Institute, University of Chicago, IL 60637, U.S.A.

[2] Department of Chemistry and Biochemistry , University of Maryland, College Park, MD 20742, U.S.A.

## I. ENTROPIC DISTANCE FUNCTION $D_e[\vec{p}(t); T_b]$

Here we show that $D_e[\vec{p}(t); T_b]$, defined by Eq. 4 in the main text, is the total entropy production of the system plus the environment along the relaxation process from $\vec{p}(t)$ at time $t$ to the final equilibrium $\vec{\pi}(T_b)$ at $t = \infty$. For simplicity, we choose a unit system where $k_B = 1$.

In stochastic thermodynamics, the total entropy production rate of a system $\vec{p}$ and the heat bath is given by [1, 2]

$$\dot{S}(t) \;=\; \sum_{i<j}(R_{ij}p_j - R_{ji}p_i)\ln\frac{R_{ij}p_j}{R_{ji}p_i}. \tag{1}$$

According to this definition, $\dot{S}$ is non-negative because the signs of $R_{ij}p_j - R_{ji}p_i$ and $\ln(R_{ij}p_j)/(R_{ji}p_i)$ are always identical. When the system is in the thermal equilibrium $\vec{p}(t) = \vec{\pi}(T_b)$, there is no entropy production and $\dot{S}$ equals zero (the system is detailed balanced). The distance function $D_e[\vec{p}(t); T_b]$ can be obtained by integrating $\dot{S}$ from time $t$ to $\infty$:

$$D_e[\vec{p}(t); T_b] = \int_t^{\infty} \dot{S}\,(t')\,dt'. \tag{2}$$

Let us denote the net probability current from state $j$ to state $i$ by

$$J_{ij} = R_{ij}p_j - R_{ji}p_i = -J_{ji} \tag{3}$$

and formulate $\dot{p}_i$ by

$$\dot{p}_i = \sum_j J_{ij} \quad . \tag{4}$$

Substituting Eq.1 into Eq.2 gives

$$\begin{aligned}
D_e[\vec{p}(t); T_b] &= \int_t^{\infty}\sum_{i<j} J_{ij}\ln\frac{R_{ij}p_j}{R_{ji}p_i}dt' = \int_t^{\infty}\sum_{i<j} J_{ij}\left(\ln p_j - \ln p_i + \frac{E_j - E_i}{T_b}\right)dt' \\
&= \int_t^{\infty}\sum_i -\dot{p}_i\ln p_i - \frac{\dot{p}_i E_i}{T_b}dt' \\
&= -\sum_i \frac{(\pi_i - p_i)E_i}{T_b} + \int_t^{\infty}\dot{p}_i\ln p_i dt' \\
&= -\sum_i \frac{(\pi_i - p_i)E_i}{T_b} + \int_t^{\infty}\frac{d}{dt}(p_i\ln p_i) - \dot{p}_i dt' \\
&= -\sum_i \frac{(\pi_i - p_i)E_i}{T_b} + \pi_i\log\pi_i - p_i\ln p_i - \pi_i + p_i \\
&= \sum_i \frac{(p_i - \pi_i)E_i}{T_b} + p_i\ln p_i - \pi_i\log\pi_i
\end{aligned} \tag{5}$$

where we used integration by parts and $\sum_i p_i = \sum_i \pi_i = 1$.

In stochastic thermodynamics, the above result has a simple interpretation [2]. The first term, $\sum_i \frac{(p_i-\pi_i)E_i}{T_b}$, is the entropy production in the bath. The second and third terms, $\sum_i(p_i\ln p_i - \pi_i\log\pi_i)$ are the changes in the Shannon entropy of the system. Generalization of the above to continuous systems is straightforward.

## II. THE DISTANCE FROM EQUILIBRIUM GROWS WITH THE INITIAL TEMPERATURE

Here we show that $D_e[\vec{\pi}(T_c);T_b] < D_e[\vec{\pi}(T_h);T_b]$ for any $T_h > T_c > T_b$. In other words, the distance function we chose has the property that the hot system starts at a greater initial distance from equilibrium at $T_b$ compared with the colder system. Notice that initially, both the hot and the cold systems start from a Boltzmann distribution at initial temperature $T_{ini} = T_h$ and $T_c$, and the distance function takes the form

$$D_e[\vec{\pi}(T_{ini});T_b] = \sum_i \frac{E_i(\pi_i(T_{ini}) - \pi_i(T_b))}{T_b} + \pi_i(T_{ini})\log\pi_i(T_{ini}) - \pi_i(T_b)\log\pi_i(T_b) \tag{6}$$

and thus

$$\begin{aligned} D_e[\vec{\pi}(T_h);T_b] - D_e[\vec{\pi}(T_c);T_b] &= \sum_i \frac{E_i(\pi_i(T_h) - \pi_i(T_c))}{T_b} + \pi_i(T_h)\log\pi_i(T_h) - \pi_i(T_c)\log\pi_i(T_c) & (7)\\ &\geq \sum_i \frac{E_i(\pi_i(T_h) - \pi_i(T_c))}{T_c} + \pi_i(T_h)\log\pi_i(T_h) - \pi_i(T_c)\log\pi_i(T_c) & (8)\\ &\geq 0 & (9) \end{aligned}$$

where the second inequality is due to the non-negativity of $D_e[\vec{p};T_c]$ for any $\vec{p}$ and $T_c$ (as is shown in section I of SI). The first inequality is due to the fact that $T_c > T_b$ and that

$$\sum_i E_i(\pi_i(T_h) - \pi_i(T_c)) = \langle E\rangle_{T_h} - \langle E\rangle_{T_c} \geq 0 \tag{10}$$

Note that the above inequality is valid for $T_h > T_c > T_b$ when the system's heat capacity if non-negative. We can show that for our system of interest, the heat capacity defined as follows is non-negative:

$$\begin{aligned} \frac{\mathrm{d}\langle E\rangle_T}{\mathrm{d}T} &= \frac{\mathrm{d}}{\mathrm{d}T}\frac{\sum_i E_i e^{-E_i/T}}{Z(T)} & (11)\\ &= \frac{\langle E^2\rangle_T - \langle E\rangle_T^2}{T^2} & (12) \end{aligned}$$

where

$$Z(T) = \sum_i e^{\frac{-E_i}{T}} \tag{13}$$

is the partition function.

This proof guarantees that the distance function of the initially hotter system always starts at a higher value compared to that of the initially colder system.

## III. THE CHOICE OF $D[\vec{p}, T_b]$ IS NOT UNIQUE.

In the main text we gave an argument showing that the Mpemba effect should occur when $\lambda_2$ is strictly larger than $\lambda_3$ and $|a_2^h| < |a_2^c|$. Here we give a more careful derivation of the same argument, using the three properties we demand from the distance-from-equilibrium function. This allows us to characterize the Mpemba effect with any good choice of distance function $D[\vec{p}, T_b]$. First, we note that

$$\vec{p}(t) = \vec{\pi}(T_b) + e^{\lambda_2 t}a_2\vec{v}_2 + ... + e^{\lambda_n t}a_n\vec{v}_n. \tag{14}$$

For large enough $t$, the terms $e^{\lambda_3 t}a_3\vec{v}_3 + ... + e^{\lambda_n t}a_n\vec{v}_n$ are exponentially smaller than $e^{\lambda_2 t}a_2\vec{v}_2$. Hence, we can expand $D[\vec{p}(t), T_b]$ around $e^{\lambda_2 t}a_2\vec{v}_2$:

$$D[\vec{p}(t), T_b] \approx D[\vec{\pi}(T_b) + e^{\lambda_2 t}a_2\vec{v}_2, T_b] + \sum_i a_i e^{\lambda_i t}\vec{v}_i \cdot \nabla D[\vec{\pi}(T_b) + e^{\lambda_2 t}a_2\vec{v}_2, T_b] \tag{15}$$

Let us next look on the difference $D[\vec{p}^h(t), T_b] - D[\vec{p}^c(t), T_b]$. Using the above expansion, we can approximate the difference as:

$$\begin{aligned} D[\vec{p}^h(t), T_b] - D[\vec{p}^c(t), T_b] &\approx D[\vec{\pi}(T_b) + e^{\lambda_2 t}a_2^h\vec{v}_2, T_b] - D[\vec{\pi}(T_b) + e^{\lambda_2 t}a_2^c\vec{v}_2, T_b]\\ &+ \sum_i e^{\lambda_i t}\left(a_i^h\vec{v}_i \cdot \nabla D[\vec{\pi}(T_b) + e^{\lambda_2 t}a_2^h\vec{v}_2, T_b] - a_i^c\vec{v}_i \cdot \nabla D[\vec{\pi}(T_b) + e^{\lambda_2 t}a_2^c\vec{v}_2, T_b]\right) & (16) \end{aligned}$$

But at large enough $t$, the term $(a_2^h - a_2^c)e^{\lambda_2 t}$ is also very small, therefore we can further expand

$$D[\vec{\pi}(T_b) + e^{\lambda_2 t}a_2^h\vec{v}_2, T_b] - D[\vec{\pi}(T_b) + e^{\lambda_2 t}a_2^c\vec{v}_2, T_b] \approx \vec{v}_2 \cdot \nabla D[\vec{\pi}(T_b) + e^{\lambda_2 t}a_2^c\vec{v}_2, T_b](a_2^h - a_2^c)e^{\lambda_2 t}. \tag{17}$$

Substituting Eq.(17) in Eq.(16) gives:

$$\begin{aligned} D[\vec{p}^h(t), T_b] - D[\vec{p}^c(t), T_b] \;&\approx\; \vec{v}_2 \cdot \nabla D[\vec{\pi}(T_b) + e^{\lambda_2 t}a_2^c\vec{v}_2, T_b](a_2^h - a_2^c)e^{\lambda_2 t} \\ &+ \sum_i e^{\lambda_i t}\left(a_i^h\vec{v}_i \cdot \nabla D[\vec{\pi}(T_b) + e^{\lambda_2 t}a_2^h\vec{v}_2, T_b] - a_i^c\vec{v}_i \cdot \nabla D[\vec{\pi}(T_b) + e^{\lambda_2 t}a_2^c\vec{v}_2, T_b]\right) \end{aligned} \tag{18}$$

The first term, $\vec{v}_2 \cdot \nabla D[\vec{\pi}(T_b) + e^{\lambda_2 t}a_2^c\vec{v}_2, T_b](a_2^h - a_2^c)e^{\lambda_2 t}$ is positive since $a_2^h > a_2^c$ and since the distance grows in the $\vec{v}_2$ direction. This can be seen by applying on the initial condition $\vec{p} = \vec{\pi}(T_b) + e^{\lambda_2 t}a_2^c\vec{v}_2$ the demand that the distance-from-equilibrium is monotonically decreasing with time. The second term (the sum in the right hand side of the above equation) might be negative, but it is proportional to $e^{\lambda_i t}$ and hence it is negligible compared to the first term which is proportional to $e^{\lambda_2 t}$. One might worry that in the $t \to \infty$ the pre-factor of $e^{\lambda_2 t}$, given by $\vec{v}_2 \cdot \nabla D[\vec{\pi}(T_b) + e^{\lambda_2 t}a_2^c\vec{v}_2, T_b]$, decays exponentially faster than the pre-factor of $e^{\lambda_i t}$ (given by $\left(a_i^h\vec{v}_i \cdot \nabla D[\vec{\pi}(T_b) + e^{\lambda_2 t}a_2^h\vec{v}_2, T_b] - a_i^c\vec{v}_i \cdot \nabla D[\vec{\pi}(T_b) + e^{\lambda_2 t}a_2^c\vec{v}_2, T_b]\right)$), and hence the $e^{\lambda_i t}$ factors cannot be neglected. However, this cannot be the case since we demand the distance function is convex, hence $\nabla D[\vec{\pi}(T_b) + e^{\lambda_2 t}a_2^h\vec{v}_2, T_b]$ approaches zero at most linearly with $e^{\lambda_2 t}$.

## IV. THE MPEMBA EFFECT IN 1-DIMENSIONAL CONFIGURATION SPACE

In the main text we gave a numerical example for the Mpemba effect in continuous configuration space, solved by the Fokker-Planck diffusion operator (see also Fig. (1b) in the main text). Here we discuss this example in detail. To this end we consider the diffusion of a Brownian particle in a potential $V(x)$ (heat bath's temperature is $T_b$). The probability to find the Brownian particle in position $x$ at time $t$ is given by $p(x,t)$, which evolves according to

$$\partial_t p(x,t) = \partial_x\Big(\mu(\partial_x V) + D\partial_x\Big)p(x,t) = \mathcal{L}p \tag{19}$$

where we assume that the diffusion and mobility coefficients, $D$ and $\mu$, are homogenous in both time and space. These two coefficients are related by the Einstein-Smoluchowski relations, $D = \mu k_B T$. In the following, we assume $\mu = 1$ and $k_B = 1$, hence the Fokker-Planck equation operator is simplified into

$$\mathcal{L} = \partial_x\Big((\partial_x V) + T_b\partial_x\Big). \tag{20}$$

The unique steady state (equilibrium distribution) of $\mathcal{L}$ is given by the Boltzmann distribution,

$$\pi(x) = \frac{e^{-V(x)/T_b}}{Z} \tag{21}$$

where

$$Z = \int e^{-V(x)/T_b}dx \tag{22}$$

is the partition function of the system at bath's temperature. The entropic distance function is given by

$$D[\vec{p}(t); T_b] = \int\left(\frac{V(x)(p(x) - \pi(x))}{T_b}\right) + p(x)\ln p(x) - \pi^b(x)\ln\pi^b(x)dx. \tag{23}$$

In the specific example we used the potential

$$\begin{aligned} V(x) \;=\;& 3\left(\arctan(x-11) - \arctan(x-9)\right) \\ &+3.1\left(\arctan(x-31) - \arctan(x-29)\right) \\ &+0.2\left(\arctan(x-70) - \arctan(x-20) + 0.05x\right) \end{aligned} \tag{24}$$

The term in the first line generate a well around $x = 10$, the second one a slightly deeper well at $x = 30$, and the third line extend the basin of the deeper well. This potential is plotted in the upper left panel of Fig(1).

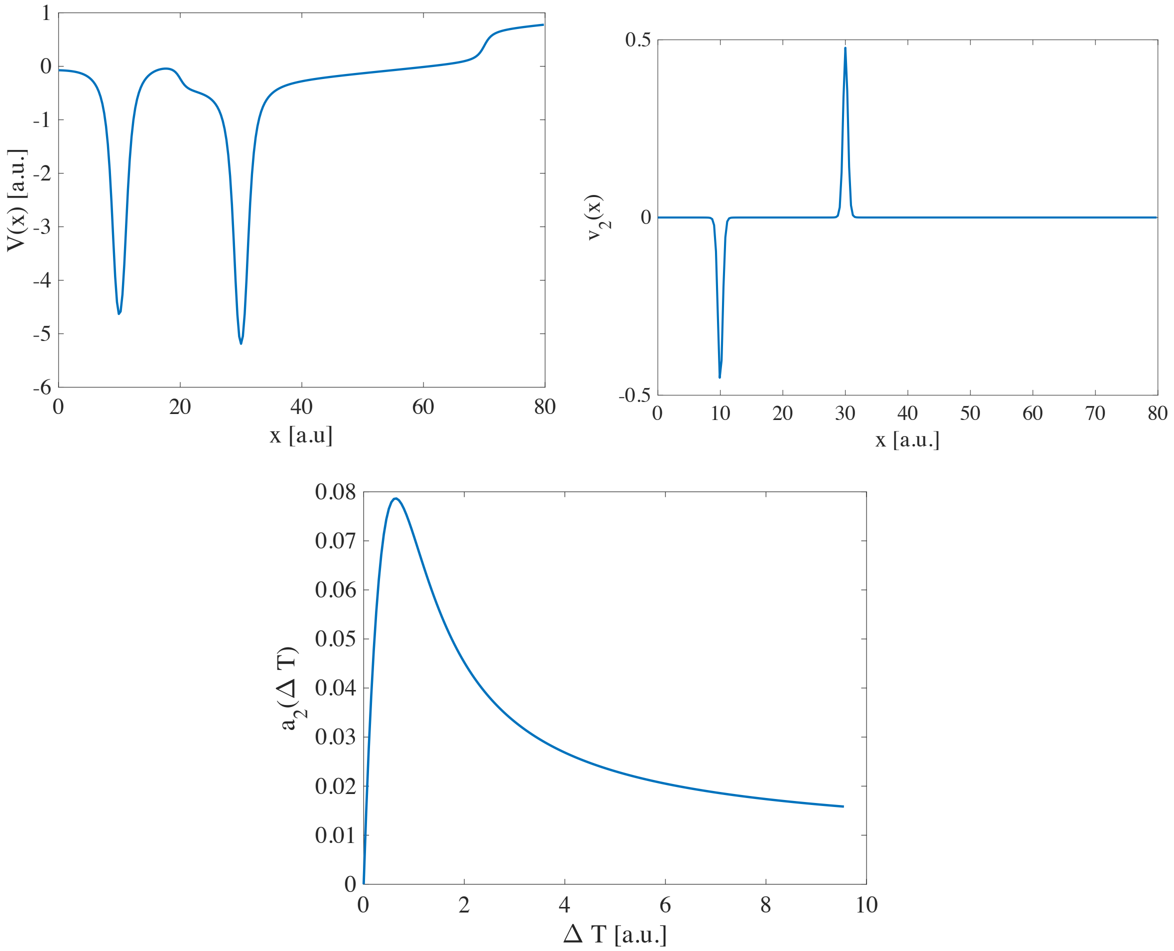


FIG. 1: **Mpemba effect in Diffusion Process:** The upper-left panel shows the potential energy landscape. The smallest nonzero eigenvalue eigenfunction is plotted on the left. As can be seen, it corresponds to a flow from one well to the other. Lower pannel - the coefficient of the smallest non-zero eigenvalue eigenfunction in the Boltzmann distribution as a function of the temperature difference from $T_b$. The coefficient decreases at high temperature, hence the Mpemba effect appears.

When two systems initially prepared at the equilibriums of $T_c = 1.38$ and $T_h = 10$, are simultaneously cooled by a bath at $T_b = 0.45$, they demonstrates the Mpemba effect (see Fig. (1c) of main text). The cooling relaxation is numerically simulated by discretizing the $x$-axis into 1000 points and integrating over time. The slowest relaxation mode, $v_2(x)$, is shown in Fig. (1) of the SI. As expected, it corresponds to a slow transition from one well into the other one. $a_2(\Delta T)$, which is the contra-variant coefficients of $\vec{v}_2(x)$ in a points along the quasi-static locus with temperature $T_b + \Delta T$, is plotted in the lower panel of Fig.(1). As can be seen, it decreases beyond some $\Delta T$, hence the Mpemba effect appears.

## V. IS IT DIFFICULT TO CONSTRUCT A 3-STATES SYSTEM WITH THE MPEMBA EFFECT?

In the main text, we provided a sufficient condition for the Mpemba effect (i.e. $a_2^h < a_2^c$) and an example with a 3-state model. One may be curious how common can an arbitrary 3-state system allows the Mpemba effect. Here we show that it it not difficult to construct such a 3-state system. In our view, the Mpemba effect is a property of the system itself: we consider a system, characterized by a set of energies $E_i$ and barriers $B_{ij}$, and ask if there exist three temperatures $T_b < T_c < T_h$, such that the Mpemba effect occurs. In the following we would like to understand in what fraction of the 3-state model parameter-space ($E_i$ and $B_{ij}$), the Mpemba effect can occur for some $T_b < T_c < T_h$. As we demonstrate below, the Mpemba effect is not restricted to a carefully chosen set of parameters, on the contrary: there exist a wide range of values in the parameter space that allows for the Mpemba effect.

For the sake of argument, we consider the limit of $T_b \to 0$. Without lose of generality, we further reduce the

parameter space by setting $E_1 = 0$, $E_3 = 1$ and $E_2 = E$ where $0 < E < 1$. With these choices (which amounts to choosing units of time and energy), the final equilibrium state is given by $\vec{v}_1 = \vec{\pi}(0) = (1,0,0)$, since at zero temperature the system is to be found only at the lowest energy state. Furthermore, in the limit of $T_b \to 0$, all the element of $R_{ij}$ are negligible except for the dominant off-diagonal element, i.e. the one with the smallest activation energy $B_{ij} - E_j$. Therefore, depending on the position of the dominant off-diagnal element, the transition rate matrix $R$ is proportional to one of the following matrices:

$$A = \begin{pmatrix} 0 & 1 & 0 \\ 0 & -1 & 0 \\ 0 & 0 & 0 \end{pmatrix}; \; B = \begin{pmatrix} 0 & 0 & 1 \\ 0 & 0 & 0 \\ 0 & 0 & -1 \end{pmatrix}; \; C = \begin{pmatrix} 0 & 0 & 0 \\ 0 & 0 & 1 \\ 0 & 0 & -1 \end{pmatrix} \tag{25}$$

Each of these matrices has a fast relaxation direction corresponding to the $\lambda_3 = -1$ eigenvalue: (i)When $B_{12} < B_{13}$ and $B_{12} - E < B_{23} - 1$, all the elements in $R$ are negligible except for $R_{12}$ and $R_{22}$, and thus $R$ is proportional to the matrix $A$ above, and $\vec{v}^3 = (1,-1,0)$. In this case $a_2^h > a_2^c$ for all $T_h$ and $T_c$, and there is no Mpemba effect. (ii) When $B_{23} < B_{13}$ and $B_{23} - 1 < B_{12} - E$, the matrix $R$ is proportional to the matrix $B$ above, and $\vec{v}^3 = (0,1,-1)$. In this case $a_2^h > a_2^c$, and there is no Mpemba effect. (iii) When $B_{13} - 1 < B_{12} - E$ and $B_{13} < B_{23}$, the matrix $R$ is proportional to the matrix $C$ above, and $\vec{v}^3 = (1,0,-1)$ . In this case there is a Mpemba effect if the curve $\vec{\pi}(T)$ is tangent to $\vec{v}^3$, which is the case when $E < \frac{1}{2}$. Therefore, in any system at which

$$E < \frac{1}{2}; \tag{26}$$

$$B_{13} - 1 < B_{12} - E; \tag{27}$$

$$B_{13} < B_{23} \tag{28}$$

the Mpemba effect occurs for sufficiently low $T_b$.

This shows that the Mpemba effect can be found in a wide range of parameters $E$ and $B_{ij}$. Consider randomly picking values of $E$, and $B_{ij}$'s uniformly from the range $(0,1)$, the chance that the above three equations holds (i.e. there exist $T_h > T_c$ where the Mpemba effect occurs) is at least 1/8: If $E$ is sampled from the interval $(0,1)$ with uniform distribution then the probability for the first condition $E < \frac{1}{2}$ is 0.5. Similarly if the $B_{ij}$'s are sampled from some interval with identical uniform distribution, then the probability for $B_{13} < B_{23}$ is 0.5, and the probability for $B_{13} - 1 < B_{12} - E$ is larger than 0.5. If all these parameters are independent, then the probability that the system is compatible with the Mpemba effect is therefore at least $\frac{1}{8}$. This calculation is clearly only a lower bound, since we only considered a single temperature, $T_b = 0$. In principle it is possible that at other values of $T_b$ there are cases with the Mpemba effect outside the range discussed above, hence the probability can be larger.

[1] J. Schnakenberg, Reviews of Modern physics **48**, 571 (1976).
[2] U. Seifert, Reports on Progress in Physics **75**, 126001 (2012).
